# Supplementary material for: Imaging molecular orbitals with laser-induced electron tunneling spectroscopy
Source: arXiv:2304.06268 ancillary file (2023-04-13)
Supplement: Supplementary file 1 [file Supplemental_materials.pdf]

*Supplemental materials for*

# Imaging molecular orbitals with laser-induced electron tunneling spectroscopy

XuanYang Lai, RenPing Sun, ShaoGang Yu, YanLan Wang, Wei Quan, André Staudte, XiaoJun Liu

## 1. Experimental setup

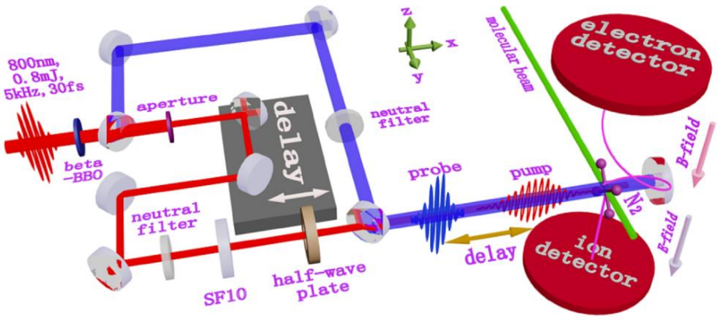


**Fig. S1:** Experimental setup. An 800 nm, 0.8 mJ, 5 kHz, 30 fs laser pulse is frequency doubled by a -BBO crystal. The two-color laser fields are then split into an 800 nm alignment pulse and a 400 nm probe pulse. The two pulses are focused into a supersonically cooled gas jet of molecule $N_2$ in the apparatus of COLTRIMS. The probe pulse, which is applied after a time delay, ionizes the molecules aligned by the alignment pulse.

## 2. Relative phase between the transition amplitudes of the different atomic orbitals

To understand the interference patterns in the photoelectron angular distributions (PADs), we analyze the relative phase between the transition amplitudes of the 2*s* and 2*p* orbitals of HOMO in $N_2$. For simplicity, we extract the terms relevant to the atomic orbitals from the transition amplitude in Eq. (2) of the main text:

$$c_a \left\langle \mathbf{Q}(t_0) \middle| \mathbf{r} \cdot \mathbf{E}(t_0) \middle| \psi_a \right\rangle \left[ e^{i\mathbf{p}\cdot\mathbf{R}/2} + (-1)^{l_a} e^{-i\mathbf{p}\cdot\mathbf{R}/2} \right] \tag{S1}$$

where $\mathbf{Q}(t_0) \equiv \mathbf{q}(t_0) + \mathbf{A}(t_0)$ denotes the initial momentum at the tunneling time $t_0$. According to the saddle-point equation [1], $Q(t_0)^2 = -2I_p$ with the ionization potential $I_p$ of an atom or a molecule. By expanding the atomic orbital $\psi_a$ with a Gaussian basis set, we obtain the expanded expressions of Eq. (S1) for the perpendicular and parallel alignments, respectively.

Firstly, for the perpendicular alignment, Eq. (S1) can be expressed as

$$-i\,c_{2s}\cos\left[p_x R/2\right]e^{-Q^2/(4\varsigma_{2s})}E_z Q_z \pi^{3/2}/(2\varsigma_{2s}{}^{5/2}) \tag{S2}$$

for the 2*s* atomic orbitals and

$$-i\,c_{2p}\sin\left[p_x R/2\right]e^{-Q^2/(4\varsigma_{2p})}E_z Q_z p_x \pi^{3/2}/(2\varsigma_{2p}{}^{5/2}) \tag{S3}$$

for the 2*p* atomic orbitals. Here, we assume that the electric field of the laser field is along the *z* direction. $Q_z$ denotes the photoelectron momentum at the time $t_0$ along the *z* direction and $p_x$ denotes the final momentum of the photoelectron along the *x* direction. Considering that the coefficients $\varsigma_{2s}$ and $\varsigma_{2p}$ in the Gaussian basis are positive real numbers and the value of $p_x$ is small and real, it can be found that the relative phase between the two equations is determined by the coefficients $c_{2s}$ and $c_{2p}$. Therefore, the phase difference between the transition amplitudes of the $2s$ and $2p$ orbitals, $\arg[M(\mathbf{p})_{2s}]-\arg[M(\mathbf{p})_{2p}]$, corresponds to the relative phase between $c_{2s}$ and $c_{2p}$.

Secondly, for the parallel alignment, Eq. (S1) can be written as

$$-i\,c_{2s}\cos\left[p_z R/2\right]e^{-Q^2/(4\varsigma_{2s})}E_z \pi^{3/2} Q_z/(2\varsigma_{2s}{}^{5/2}) \tag{S4}$$

for the $2s$ atomic orbitals and

$$-i\,c_{2p}\sin\left[p_z R/2\right]e^{-Q^2/(4\varsigma_{2p})}E_z \pi^{3/2}\left[Q_z^2/(4\varsigma_{2p}{}^{7/2})-1/(2\varsigma_{2p}{}^{5/2})\right] \tag{S5}$$

for the $2p$ atomic orbitals. Similarly, by comparing with the two equations, we find that the momentum $Q_z$ along the laser polarization, which is purely imaginary according to the saddle-point equation [1], will also make effect in the relative phase. Therefore, besides the coefficients $c_{2s}$ and $c_{2p}$, an additional phase of $\pi/2$ contributes to the phase difference between the transition amplitudes of the 2*s* and 2*p* orbitals.

## 3. M-CQSFA-simulated PAD of a larger molecule

Here, we also simulate the PAD of a larger molecule, i.e., $N_2H_2$, or Diazene. For better comparison with the PAD of the simple molecule $N_2$, we consider the HOMO-2 of $N_2H_2$ (shown in Fig. 2S(a)), which has the same $\sigma_g$ symmetry as the HOMO of $N_2$. Fig. 2S(b) shows the simulated PAD of $N_2H_2$ with the M-CQSFA theory, in which a rich interference pattern can be observed. For example, there are four peculiar peaks off the white dashed curve with the momentum of $|p|$ = 0.5 a.u., which are marked by four arrows in the PAD. The two peaks marked by the red arrows can be found in the PAD of two N atoms, shown in Fig. 2S(c). Their energy shift originates from the interference of the *s* and *p* atomic orbitals of the two N atoms. On the other side, the two peaks marked by the blue arrows can be observed in PAD of two H atoms in Fig. 2S(d) and the energy shift is due to the two-center interference from two *s* orbitals of the two H atoms [2]. The use of these peculiar interference features in the PADs will benefit the accurate reconstruction of more complicated molecular orbital with our imaging method.

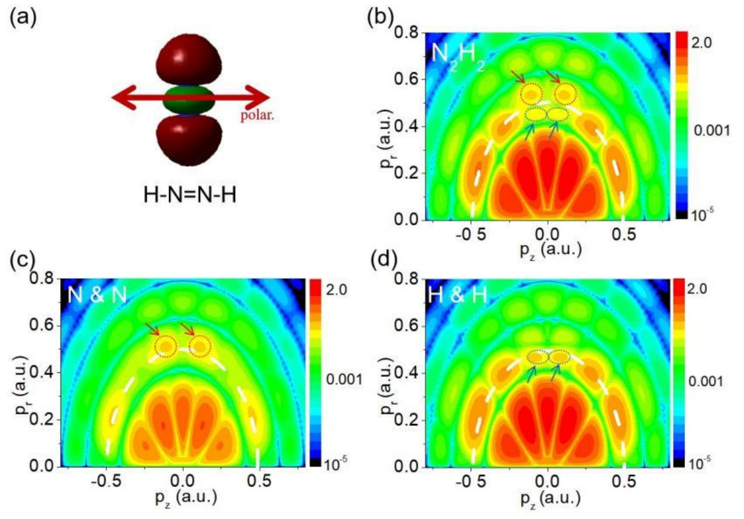


**Fig. 2S:** (a) Schematic view of the strong-field ionization of the molecule $N_2H_2$ in HOMO-2 with $\sigma_g$ symmetry. The laser polarization is perpendicular to the molecular axis. (b) Simulated PADs of $N_2H_2$ with the M-CQSFA theory, in which four peculiar peaks are marked by four arrows. (c) and (d) M-CQSFA simulated PADs from two N atoms and two H atoms, respectively.

## References:


[1] W. Becker, *et al*. Above-threshold ionization: From classical features to quantum effects. Adv. At. Mol. Opt. Phys. **48**, 35 (2002).

[2] M. Busuladžić, *et al.* Angle-Resolved High-Order Above Threshold Ionization of a Molecule: Sensitive Tool for Molecular Characterization, Phys. Rev. Lett. **100**, 203003 (2008).
